# Supplementary material for: BNN-DP: Robustness Certification of Bayesian Neural Networks via Dynamic Programming
Source: arXiv:2306.10742 source file (2023-06-19)
Supplement: Supplementary file 1 [file linear_relaxations.tex]

%% Non-used props. Can be used to perform linear relaxation of the probability term. 
%% Need to check performence difference compared to linear relaxation

\begin{proposition}\label{prop:CombinePWABounds}
    Let $f_1,f_2:\mathbb{R}\rightarrow\mathbb{R}$ be affine functions $f_1=A_1x+b_1$ and $f_2=A_2x+b_2$ with $A_1,A_2\in\mathbb{R}^{1\times 1}$ and $b_1,b_2]\in\mathbb{R}$ defined over domains $[\check{x}_1,\hat{x}_1]\subset\mathbb{R}$ and $[\hat{x}_1,\hat{x}_2]\subset\mathbb{R}$, respectively. Then 
    \begin{align*}
        xx
    \end{align*}
    
    \SA{to do..}
\end{proposition}

\begin{proposition}\label{prop:LBSemiDefQuad}
    Let $f:\mathbb{R}^n\rightarrow\mathbb{R}$ be a quadratic function $f(x)=x^TQx$ with $Q\in\mathbb{R}^{n\times n}$ a semi-definite matrix. \SA{to do..}
\end{proposition}

\begin{proposition}\label{prop:LBConvConvexFuncs}
    Let $f:\mathbb{R}^n\rightarrow\mathbb{R}$ be a convex function. \SA{to do..}
\end{proposition}

\begin{proposition}\label{prop:LBDivision}
    Let $\gamma:\mathbb{R}^2\rightarrow\mathbb{R}$, $\gamma=\frac{\mu}{\sigma}$, and $\mu\in[\check{\mu},\hat{\mu}]\subseteq\mathbb{R}$ and $\sigma\in [\check{\sigma},\hat{\sigma}]\subseteq \mathbb{R}_{\geq0}$. Then, 
    $$\vecCoefL^T \mat{c}{\mu \\ \sigma} + \biasL \leq f(\mu,\sigma) \leq \vecCoefU^T \mat{c}{\mu \\ \sigma} + \biasU $$
    where
    \begin{align*}
        \vecCoefL &= \begin{cases}
        [\nabla\gamma(\mu,\sigma)]_{(\mu,\sigma)=(\mu^*,\sigma^*)} &\text{if} \quad
        [\check{\mu},\hat{\mu}]\subseteq\mathbb{R}_{\geq 0} \\
        \mat{cc}{\frac{\gamma(\hat{\mu}, \check{\sigma})-\gamma(\check{\mu}, \check{\sigma})}{\hat{\mu}-\check{\mu}} & \frac{\gamma(\check{\mu}, \hat{\sigma})-\gamma(\check{\mu}, \check{\sigma})}{\hat{\sigma}-\check{\sigma}}}^T &\text{else if} \quad
        [\check{\mu},\hat{\mu}]\subseteq\mathbb{R}_{< 0} \\
        \mat{cc}{\frac{\gamma(0, \check{\sigma})-\gamma(\check{\mu}, \check{\sigma})}{-\check{\mu}} & \frac{\gamma(\check{\mu}, \hat{\sigma})-\gamma(\check{\mu}, \check{\sigma})}{\hat{\sigma}-\check{\sigma}}}^T &\text{else} \\
        \end{cases}\\
        \biasL &= \begin{cases}
        \gamma(\mu^*, \sigma^*) - \vecCoefL \mat{cc}{\mu & \sigma}^T &\text{if} \quad [\check{\mu},\hat{\mu}]\subseteq\mathbb{R}_{\geq 0} \\
        \gamma(\check{\mu}, \hat{\sigma}) - \vecCoefL \mat{cc}{\check{\mu} & \hat{\sigma}}^T &\text{else}
        \end{cases}\\
        \vecCoefU &= \begin{cases}
        \mat{cc}{\frac{\gamma(\hat{\mu}, \check{\sigma})-\gamma(\check{\mu}, \check{\sigma})}{\hat{\mu}-\check{\mu}} & \frac{\gamma(\hat{\mu}, \hat{\sigma})-\gamma(\hat{\mu}, \check{\sigma})}{\hat{\sigma}-\check{\sigma}}}^T&\text{if} \quad
        [\check{\mu},\hat{\mu}]\subseteq\mathbb{R}_{\geq0} \\
        [\nabla\gamma(\mu,\sigma)]_{(\mu,\sigma)=(\mu^*,\sigma^*)} &\text{else if} \quad
        [\check{\mu},\hat{\mu}]\subseteq\mathbb{R}_{<0} \\
        \mat{cc}{\frac{\gamma(\hat{\mu}, \check{\sigma})-\gamma(0, \check{\sigma})}{\hat{\mu}} & \frac{\gamma(\hat{\mu}, \hat{\sigma})-\gamma(\hat{\mu}, \check{\sigma})}{\hat{\sigma}-\check{\sigma}}}^T &\text{else} \\
        \end{cases}\\
        \biasU &= \begin{cases}
        \gamma(\mu^*, \sigma^*) - \vecCoefL \mat{cc}{\mu & \sigma}^T &\text{if} \quad
        [\check{\mu},\hat{\mu}]\subseteq\mathbb{R}_{<0} \\
        \gamma(\hat{\mu}, \hat{\sigma}) - \vecCoefL \mat{cc}{\hat{\mu} & \hat{\sigma}}^T &\text{else}
        \end{cases}
    \end{align*}
    with $(\mu^*, \sigma^*)\in [\check{\mu},\hat{\mu}]\times [\check{\sigma}, \hat{\sigma}]$
\end{proposition}

\begin{proposition}\label{prop:LBErf}
    Let $\text{erf}:\mathbb{R}\rightarrow\mathbb{R}$ be the error function. Then, \SA{todo..}
    \begin{align*}
        \erf{x} & \geq \begin{cases} 
        &\text{if} \quad x\in\mathbb{R}_{\leq0}\\
        &\text{else if} \quad x\in\mathbb{R}_{>0}\\
        &\text{else}\\
        \end{cases}\\
        \erf{x} & \leq \begin{cases} 
        &\text{if} \quad x\in\mathbb{R}_{\leq0}\\
        &\text{else if} \quad x\in\mathbb{R}_{>0}\\
        &\text{else}\\
        \end{cases}
    \end{align*}
    
\end{proposition}
