# Supplementary material for: BNN-DP: Robustness Certification of Bayesian Neural Networks via Dynamic Programming
Source: arXiv:2306.10742 source file (2023-06-19)
Supplement: Supplementary file 2 [file results.tex]

\subsection{Regression}

% \begin{figure*}[t]
%     \centering
%     \begin{subfigure}{0.7\textwidth}
%         \centering
%         \includegraphics[width=0.32\textwidth]{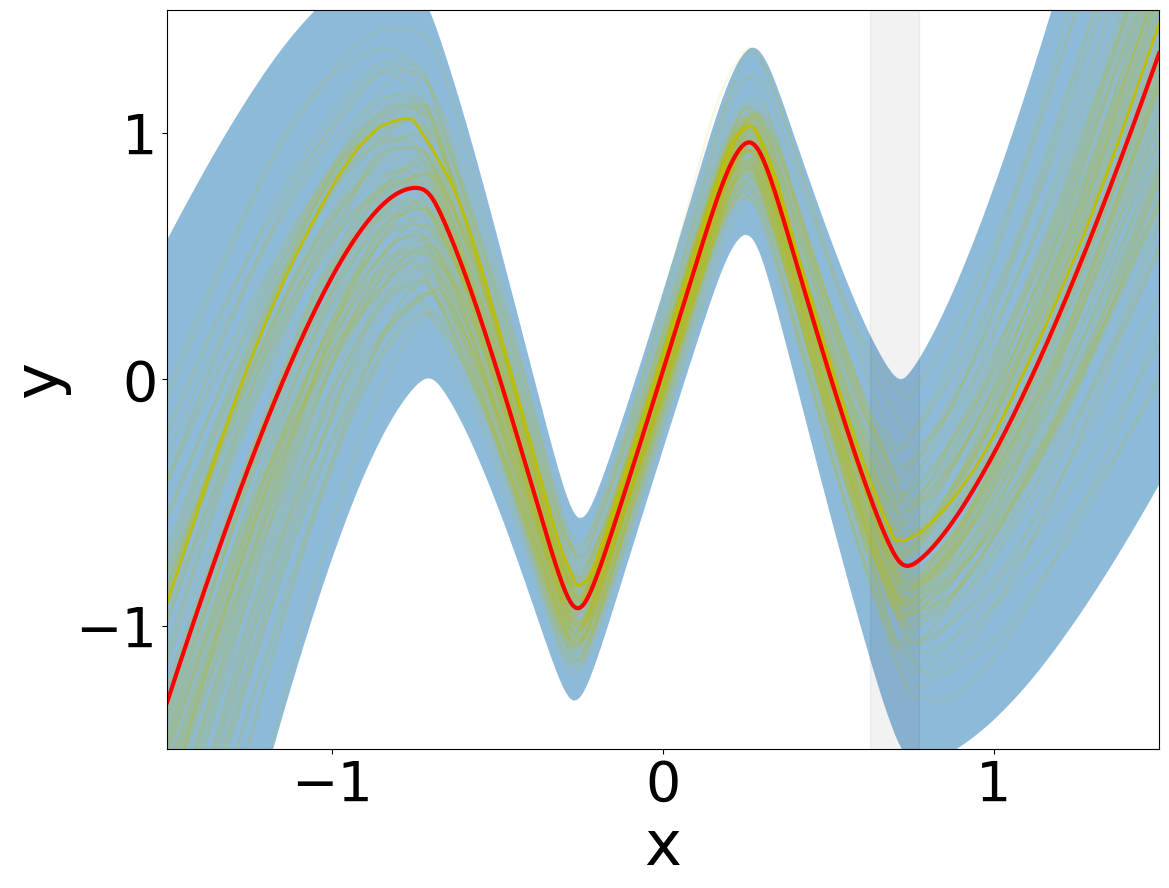}
%         \includegraphics[width=0.32\textwidth]{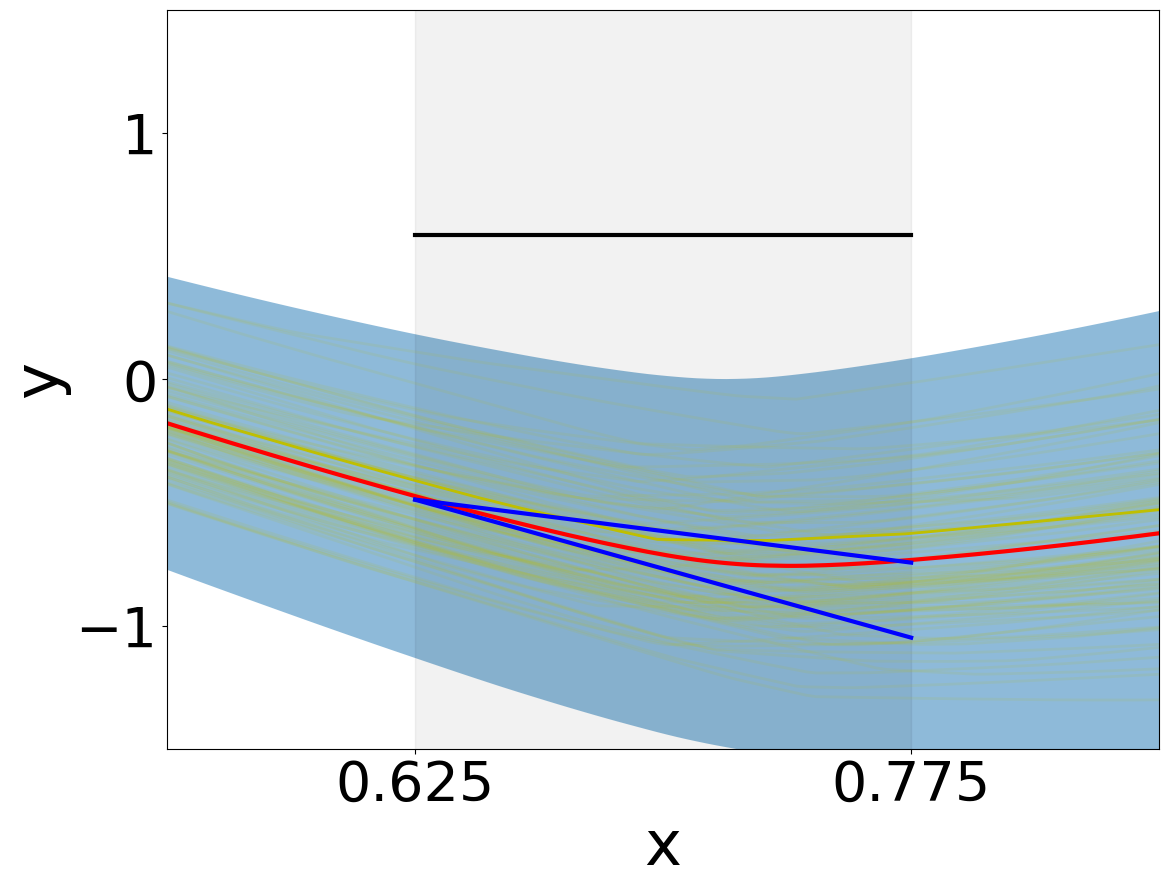}
%         \includegraphics[width=0.32\textwidth]{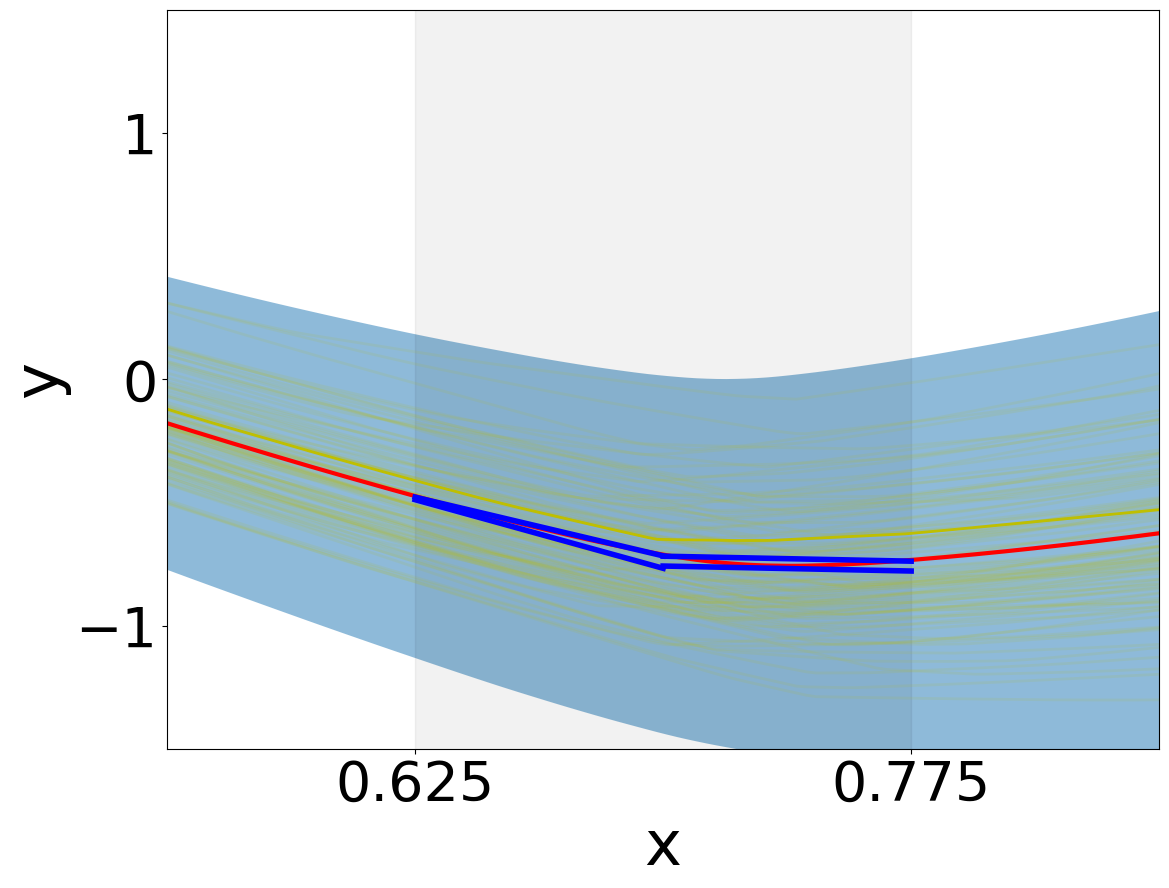}
%         \caption{BNN with 1 hidden layer and 2048 nodes. }
%         \label{fig:Noisy_sine_1/hid=2048_arch=fc1}
%     \end{subfigure}
%     \begin{subfigure}[t]{0.1\textwidth}
%             \centering
%             \includegraphics[width=0.97\textwidth]{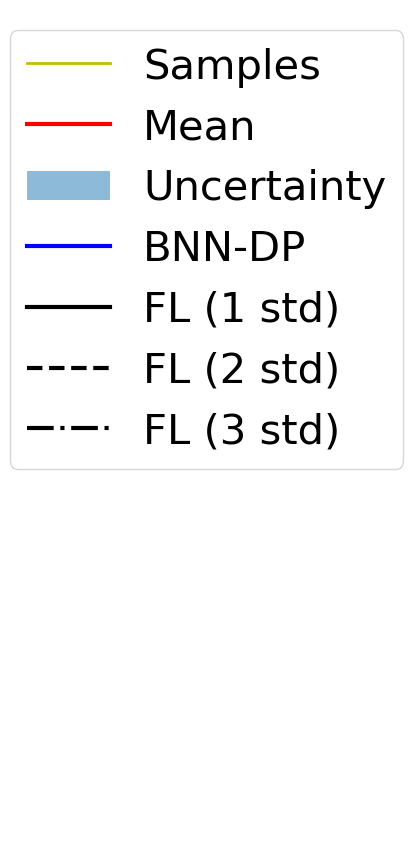}
%     \end{subfigure}
%     \caption{Certified affine bounds on the mean of BNNs trained on the 1D Noisy Sine dataset w.r.t. the grey marked interval of input. 
%     }
% \end{figure*}

\begin{table}[H]
    \centering
    \begin{tabular}{ccc|rrr|rrr}\toprule
        \multicolumn{3}{c|}{\textbf{2D Noisy Sine}} & \multicolumn{3}{c|}{$\gamma$-Robustness} &  \multicolumn{3}{c}{Computation Time (sec)} \\ \midrule
        $K$ & $\epsilon$ & $n_{hid}$ & BNN-DP & FL (5 std) & FL (3 std) & BNN-DP  & FL (5 std) & FL (3 std) \\ \midrule 
        1 &1e-2   &       64 &  \textbf{0.041} & 1.8 &    0.8 &      \textbf{0.9} &5.9&      6.0 \\
          &       &       256&   \textbf{0.040} & 3.0 &    1.2 &      \textbf{3.8} &6.0&      6.0 \\
          &       &      512 &  \textbf{0.039} & 6.4&    2.5 &      6.9 &5.9&      \textbf{5.8} \\
        2 &1e-3   &       64 &  \textbf{0.109} & 718.1 &  101.1 &      \textbf{2.0} &7.7&      7.7 \\
         &        &      128 &  \textbf{0.239} &112.2&   20.1 &      \textbf{4.0} &7.5&      8.2 \\
         &        &      256 &  \textbf{0.376} &599.3&   92.1 &      \textbf{8.2} &7.6&      7.7 \\ 
        3 &5e-4   &       64 &  \textbf{0.477} &699.2 & 74.8& 10.2 & 9.5& \textbf{9.2} \\ 
         &        &      128 & \textbf{0.629} & 11214.4 & 1142.8 & 21.2 & \textbf{9.1} & 9.4 \\ 
         &        &     256  & \textbf{14.180} & 275408.1 & 2882.3 & 19.9 & 9.5 & \textbf{9.4} \\ \midrule
        \multicolumn{3}{c}{\textbf{Kin8nm}} &&   & &   &&  \\
        1 & 1e-2 &     64 & \textbf{0.044}  &0.7&      0.3 &     \textbf{2.6} &5.8&      5.9 \\
          & &     128  &\textbf{0.045}  &3.0&     1.4 &      \textbf{5.6} &5.7&      5.9 \\
          & &     256  &\textbf{0.040}  &45.4&    24.7 &      6.4 &5.9&      \textbf{5.8} \\
          & &     512  &\textbf{0.041}  &12.6&     6.0 &    19.2 &\textbf{5.8}&       5.9 \\
        2 & 1e-3 &      64 &\textbf{0.070}  &31.3&    10.8 &     \textbf{7.7} &7.8&      7.8\\
          &      &128  &\textbf{0.240}  &1459.8&   420.9 &     18.9 &\textbf{7.4}&      7.7\\
          &      &256  &\textbf{0.968}  &9420.9&  2715.9 &     20.7 &\textbf{7.6}&      7.7\\
        3 &5e-4  &64   &\textbf{0.348}  &12638.5& 59304.6 & 10.4 & 9.4 & \textbf{9.2} \\
          &      &128  &\textbf{0.964}  &433149.4& 232811.6 & 21.4 & \textbf{9.1} & 9.2  \\
          &      &256  &\textbf{69.488}  &3441470.8 & 21877545.4 & 11.8 & 9.2 & 9.1 \\ \bottomrule
        % \label{tab:regression}
    \end{tabular}
    \caption{Comparison for BNNs of various architecture, where $K$ is the number of hidden layers, and $n_{hid}$ is the number of neurons per hidden layer, of the differences between the upper and lower bounds ($\gamma$) on the expectations of various BNNs for the input being in an $\ell_{\infty}$-norm balls of radius $\epsilon$ centered at a sampled data-point. For each architecture the results are obtained by averaging over $100$ test inputs.}
\end{table}

\subsection{Classification}
\begin{table}[H]
    \centering
        \begin{tabular}{cc|ccc|ccc}\toprule
        \multicolumn{2}{c|}{\textbf{MNIST}}& \multicolumn{3}{c|}{$\epsilon$-Robustness}& \multicolumn{3}{c}{Computation Time (sec)}\\ \midrule
         $K$ & $n_{hid}$ & BNN-DP & FL (5 std) & FL (3 std)& BNN-DP & FL (5 std) & FL (3 std) \\ \midrule 
            1 &       48 &  \textbf{0.0157} & 0.0114 &  0.0140 &     \textbf{10.0} & 804.6 &   498.0 \\
              &       64 &   \textbf{0.0150} & 0.0102  &   0.0090 &      \textbf{9.0} & 839.7 &   357.0 \\
              &      128 &  \textbf{0.0145} & 0.0091 &  0.0131 &   \textbf{6.0} & 936.9 &  1485.0 \\
              &      256 &  \textbf{0.0137} & 0.0082 &   0.0090 & \textbf{11.0} & 907.5 &   867.0\\
              &      512 & \textbf{0.0131} & 0.0070 & 0.0073 & \textbf{17.5} & 881.4 & 865.8\\
             2 &       48 &  \textbf{0.0083} & 0.0049 &  0.0052 & \textbf{3.0} & 943.5 &   942.0\\
              &       64 &  \textbf{0.0073} & 0.0042 &  0.0041 &\textbf{5.0} &891.3&   537.0\\
              &      128 &  \textbf{0.0062} & 0.0028 &  0.0035 &\textbf{9.0} &783.9&   915.0\\
              &      256 &  \textbf{0.0049} & 0.0023 &  0.0023 &\textbf{19.0} &815.3&   768.0 \\ 
             3 &      64 &  \textbf{0.0032} & 0.0014 & 0.0016 & \textbf{29.2} & 794.2& 760.5 \\
               &     256 &  \textbf{0.0018} & 0.0009 & 0.0009 & \textbf{34.3} & 876.5 & 819.7 \\ \midrule
        \multicolumn{2}{c|}{\textbf{FashionMNIST}} &   & & & & &    \\
        1 &       64 &  \textbf{0.0128} & 0.0077 &   0.008 &      \textbf{2.0} & 823.5 &   838.2 \\
          &      256 &  \textbf{0.0081} & 0.0043 &  0.0046 &      \textbf{7.5} &582.3 &   753.3 \\
          &      512 &  \textbf{0.0092} & 0.0044 &  0.0048 &     \textbf{15.1} &675.2 &   738.3\\
        2 &       64 &  \textbf{0.0048} & 0.0024 &  0.0026 &      \textbf{3.0} &535.5 &   763.2\\
          &      256 &  \textbf{0.0032} & 0.0016 &  0.0016 & \textbf{12.4} & 620.9 &   760.0 \\
        3 &     64   & \textbf{0.0015} & 0.0006 & 0.0008 & \textbf{27.8} & 815.9 & 756.3 \\
          &     256 &&&&&& \\
        \bottomrule
        % \label{tab:classification}
    \end{tabular}
    \caption{Comparison for BNNs of various architecture, where $K$ is the number of hidden layers, and $n_{hid}$ is the number of neurons per hidden layer, of the certified upper bounds on the radius $\epsilon$ of $\ell_{\infty}$-norm perturbations of images for which robust classification is guaranteed. For each architecture the results are obtained by averaging over $100$ test inputs.}
\end{table}
