# Supplementary material for: BNN-DP: Robustness Certification of Bayesian Neural Networks via Dynamic Programming
Source: arXiv:2306.10742 source file (2023-06-19)
Supplement: Supplementary file 3 [file nnCondExpect.tex]

% \section{Non-Normalized Conditional Expectation}
%% ---- OLD PRELIMS SECTION ----
% To propagate the uncertainty of the BNN from one layer to the other we first introduce several results for the so-called non-normalized conditional expectation of a random variable. Suppose we want to compute $\E{\bm{z}\sim p(z)}{l(\bm{z})}$ for $l: \mathbb{R}\rightarrow\mathbb{R}$, 
% $$
% l(z) = \begin{cases}
% a_0z + b_0& z\in Z_0\\
% a_1z+b_1 & z\in Z_1
% \end{cases}
% $$
% a piecewise affine (pwa) function, with $a_0,a_1,b_0,b_1\in\mathbb{R}, Z_0,Z_1\subset\mathbb{R}$, such that
% $$\E{\bm{z}\sim p(z)}{l(z)}=\sum_{i\in\{0,1\}} (a_i\condE{\bm{z}\sim p(z)}{\bm{z}}{\bm{z}\in Z_i} + b_i) \Prob{}{\bm{z}\in Z_i}.$$
% Here, the linear terms are multiplied by the so called non-normalized conditional expectation, defined as follows.  

% \begin{definition}[Non-normalized conditional expectation]
% For a random variable $\bz{}$ with pdf $p(z)$ and hyper-rectangle $Z\subseteq\mathbb{R}$, we define the non-normalized conditional expectation as
% $$\nncondE{p(z)}{\z{}}{\bz{}\in Z}\coloneqq \int_Z z p(z) dz$$
% \end{definition}
% In the case of $p(z)$ being an univariate Gaussian pdf, the non-normalized conditional expectation of $\bz{}\sim p(z)$ w.r.t. interval $Z$ can be expressed as the sum of expectations and probabilities of rectified Gaussian variables. 

% \begin{proposition}\label{prop:nnCondExpectGaussian}
% Let $\bz{}\sim \nDist{\mu}{\sigma^2}$ be a univariate Gaussian random variable with mean $\mu\in\mathbb{R}$ and variance $\sigma\in\mathbb{R}_{\geq 0}$. Then 
% \begin{align*}
% %   &\condE{\bz{}\sim\nDist{\mu}{\sigma^2}}{\bz{}}{\bz{}\in Z}\Prob{}{\bz{}\in Z} =
%    \nncondE{\bz{}\sim\nDist{\mu}{\sigma^2}}{\bz{}}{\bz{}\in [\check{z},\hat{z}]} &=
%    \E{\bz{}\sim\rectnDist{\mu-\check{z}}{\sigma^2}}{\bz{}} -  \E{\bz{}\sim\rectnDist{\mu-\hat{z}}{\sigma^2}}{\bz{}} + \\
%      & \check{z}\Prob{\bz{}\sim\nDist{\mu}{\sigma^2}}{\bz{}\in[\check{z},\infty)} -  \hat{z}\Prob{\bz{}\sim\nDist{\mu}{\sigma^2}}{\bz{}\in[\hat{z},\infty)}.
% \end{align*}
% \end{proposition}
% Similarly, the non-normalized conditional expectation of a rectified Gaussian variable can be expressed as the sum of expectations and probabilities of rectified Gaussian variables. 

% \begin{corollary}\label{corol:nnCondExpectRectGaussian}
% Let $\bz{}\sim \rectnDist{\mu}{\sigma^2}$ be an univariate rectified Gaussian random variable with mean $\mu\in\mathbb{R}$ and variance $\sigma\in\mathbb{R}_{\geq 0}$. Then
% \begin{align*}
%    \nncondE{\bz{}\sim\rectnDist{\mu}{\sigma^2}}{\bz{}}{\bz{}\in [\check{z},\hat{z}]} &= \nncondE{\bz{}\sim\nDist{\mu}{\sigma^2}}{\bz{}}{\bz{}\in [\check{\bar{z}},\hat{\bar{z}}]},
% \end{align*}
% where $\check{\Bar{z}} = \max(\check{z},0)$ and $\hat{\Bar{z}} = \max(\hat{z},0)$.
% \end{corollary}
% Moreover, the non-normalize expectation of (rectified) Gaussian distributed variables conditioned on unbounded regions located fully in the positive or negative space can be upper bounded by 'simple' exponential functions, as shown in the following proposition.

% \begin{proposition}\label{prop:BoundCondExpect}
% Let $\bz{}\sim\nDist{\mu}{\sigma^2}$, with $\mu\in\mathbb{R}$ and $\sigma\in\mathbb{R}_{\geq0}$. Define functions $\check{\epsilon},\hat{\epsilon}:\mathbb{R}\rightarrow\mathbb{R}$ as, 
% \begin{align*}
% \check{\epsilon}(z) = \Exp{\frac{\mu-z}{\sigma\sqrt{2\pi}}+\frac{1}{2}}\left(\frac{z}{\sigma\sqrt{2\pi}}+1\right), \qquad
% \hat{\epsilon}(z) = \Exp{\frac{z-\mu}{\sigma\sqrt{2\pi}}+\frac{1}{2}}\left(\frac{z}{\sigma\sqrt{2\pi}}+1\right)
% \end{align*}
% Then, for $\check{z}\in\mathbb{R}_{\geq 0}$ and $\hat{z}\in\mathbb{R}_{\leq 0}$, it holds that
% \begin{align*}
% \nncondE{\bz{}\sim\nDist{\mu}{\sigma^2}}{\bz{}}{\bz{}\in [\check{z},\infty)} &\leq \check{\epsilon}(\check{z}) \\
% \nncondE{\bz{}\sim\nDist{\mu}{\sigma^2}}{\bz{}}{\bz{}\in (\infty,\hat{z}]} &\leq\hat{\epsilon}(\hat{z}).    
% \end{align*}
% \end{proposition}

% \begin{corollary}\label{corol:BoundCondExpectRect}
% Let $\bz{}\sim\rectnDist{\mu}{\sigma^2}$, with $\mu\in\mathbb{R}$ and $\sigma\in\mathbb{R}^+$. Define functions $\check{\epsilon},\hat{\epsilon}:\mathbb{R}\rightarrow\mathbb{R}$ as in Proposition \ref{prop:BoundCondExpect}. Then, for $\check{z}\in\mathbb{R}^+$, it holds that
% \begin{align*}
% \nncondE{\bz{}\sim\rectnDist{\mu}{\sigma^2}}{\bz{}}{\bz{}\in [\check{z},\infty)} &\leq \check{\epsilon}(\check{z}) \\
% \nncondE{\bz{}\sim\rectnDist{\mu}{\sigma^2}}{\bz{}}{\bz{}\in (\infty,\hat{z}]} &\leq\hat{\epsilon}(\hat{z}).    
% \end{align*}
% \end{corollary}

%% ---- DEFINITION NON-NORMALIZED CONDITIONAL EXPECTATION ----
% moved to prelims

% %% ---- NON-NORMALIZED COND EXPECTATION GAUSSIAN ----
% \subsection*{Proposition \ref{prop:nnCondExpectGaussian}}
% \begin{proof}
% By definition of the non-normalized conditional expectation and the substitution rule for integration, it holds that
% \begin{align*}
%     \nncondE{\bz{}\sim\nDist{\mu}{\sigma^2}}{\bz{}}{\bz{}\in [\check{z},\hat{z}]} &= 
%     \int_{\check{z}}^{\hat{z}} z \nProbDens{z}{\mu}{\sigma^2}dz \\
%     &= \int_{\check{z}}^{\infty} z \nProbDens{z}{\mu}{\sigma^2}dz - \int_{\hat{z}}^{\infty} z \nProbDens{z}{\mu}{\sigma^2}dz \\
%     &= \int_{0}^{\infty} (z+\check{z}) \nProbDens{z+\check{z}}{\mu}{\sigma^2}dz - \int_{0}^{\infty} (z+\hat{z}) \nProbDens{z+\hat{z}}{\mu}{\sigma^2}dz \\
%     &= \int_{0}^{\infty} (z+\check{z}) \nProbDens{z}{\mu-\check{z}}{\sigma^2}dz - \int_{0}^{\infty} (z+\hat{z}) \nProbDens{z}{\mu-\hat{z}}{\sigma^2}dz \\
%     &= \E{\bz{}\sim\rectnDist{\mu-\check{z}}{\sigma^2}}{\bz{}} - \E{\bz{}\sim\rectnDist{\mu-\hat{z}}{\sigma^2}}{\bz{}} +  \\  
%     & \qquad \check{z}\Prob{\bz{}\sim\nDist{\mu-\check{z}}{\sigma^2}}{\bz{}\in[0,\infty]} -  \hat{z}\Prob{\bz{}\sim\nDist{\mu-\hat{z}}{\sigma^2}}{\bz{}\in[0,\infty]}
% \end{align*}
% \end{proof}

% %% ---- NON-NORMALIZED COND EXPECTATION RECTIFIED GAUSSIAN ----
% \subsection*{Corollary \ref{corol:nnCondExpectRectGaussian}}
% Let $\check{\Bar{z}} = \max(\check{z},0)$ and $\hat{\Bar{z}} = \max(\hat{z},0)$, then by the definition of the rectified Gaussian distribution we have
% \begin{align*}
%     \nncondE{\bz{}\sim\rectnDist{\mu}{\sigma^2}}{\bz{}}{\bz{}\in Z} &= 
%     \int_{\check{z}}^{\hat{z}} z \rectnProbDens{z}{\mu}{\sigma^2}dz \\
%     &= \int_{\check{\Bar{z}}}^{\hat{\Bar{z}}} z \nProbDens{z}{\mu}{\sigma^2}dz\\
%     &= \nncondE{\bz{}\sim\nDist{\mu}{\sigma^2}}{\bz{}}{\bz{}\in [\check{\bar{z}}, \hat{\bar{z}}]}.
% \end{align*}
% Such that we can directly apply the result of Proposition \ref{prop:nnCondExpectGaussian} to compute the non-normalized conditional expectation of an rectified Gaussian distribution.

%% ---- OUTER BOUNDS NON-NORMALIZED CONDITIONAL EXPECTATION GAUSSIAN ----
% \subsection*{Proposition \ref{prop:boundOuterSpace}}
% \begin{proof}
% % Define functions $\check{\epsilon},\hat{\epsilon}:\mathbb{R}\rightarrow\mathbb{R}$ as, 
% % \begin{align*}
% % \check{\epsilon}(z) &= \Exp{\frac{\mu-z}{\sigma\sqrt{2\pi}}+\frac{1}{2}}\left(\frac{z}{\sigma\sqrt{2\pi}}+1\right)\\
% % \hat{\epsilon}(z) &= \Exp{\frac{\mu-z}{\sigma\sqrt{2\pi}}+\frac{1}{2}}\left(\frac{z}{-\sigma\sqrt{2\pi}}+1\right)
% % \end{align*}
% By the definition of non-normalized conditional expectations and the substitution rule for integration we have
% \begin{align*}
%   \nncondE{\bz{}\sim\nDist{\mu}{\sigma^2}}{z}{z\in [\check{z},\infty]} 
%     % &= \int_{\check{z}}^{\infty} z\nProbDens{z}{\mu}{\sigma}dz \\
%     &= \int_{\check{z}}^{\infty} \frac{z}{\sigma\sqrt{2\pi}}\Exp{-\left(\frac{z-\mu}{\sigma\sqrt{2}}\right)^2}dz \\
%     &= \frac{1}{\sqrt{\pi}}\int_{\frac{\check{z}-\mu}{\sigma\sqrt{2}}}^{\infty}(q\sigma\sqrt{2}+\mu)\Exp{-q^2}dq, \\
%     &= \frac{\mu}{2}\left(1 - \erf{\frac{\check{z}-\mu}{\sigma\sqrt{2\pi}}} \right) + 
% \frac{2\sigma}{\sqrt{2\pi}}\int_{\frac{\check{z}-\mu}{\sigma\sqrt{2}}}^{\infty}q\Exp{-q^2}dq,
% \end{align*}
% Since, $\forall q \in[0,1]\ -q^2\leq -q+\frac{1}{2}$,
% $$\Exp{-q^2}\leq \Exp{-q+\frac{1}{2}}, \qquad \forall q\in \mathbb{R}$$
% Such that, for $\check{z}-\mu \geq 0$ it holds that
% \begin{align*}
%     \int_{\frac{\check{z}-\mu}{\sigma\sqrt{2}}}^{\infty}q\Exp{-q^2}dq \leq \left[-\Exp{-q+\frac{1}{2}}(q+1)\right]_{\frac{\check{z}-\mu}{\sigma\sqrt{2}}}^{\infty}
% \end{align*}
% Finally, since $\lim_{z\rightarrow\infty}\Exp{-z}z=0$, we obtain
% \begin{align*}
%     \nncondE{\bz{}\sim\nDist{\mu}{\sigma^2}}{z}{z\in [\check{z},\infty]} \leq \frac{\mu}{2}\left(1 - \erf{\Tilde{z}} \right) + \frac{2\sigma}{\sqrt{2\pi}}\Exp{-\Tilde{z} + \frac{1}{2}}\left(\Tilde{z}+1\right)
% \end{align*}
% where $\Tilde{z} = \frac{\check{z}-\mu}{\sigma\sqrt{2}}$
% \end{proof}


% %% ---- BOUNDS NON-NORMALIZED CONDITIONAL EXPECTATION RECTIFIED GAUSSIAN ----
% % moved to prelims
% \subsection*{Corollary \ref{corol:BoundCondExpectRect}}
% \begin{proof}
% For $z^L,z^U\geq 0$ we have that
% \begin{align*}
%     \nncondE{\bz{}\sim\rectnDist{\mu}{\sigma^2}}{z}{z\in [z^L,z^U]} =  \nncondE{\bz{}\sim\nDist{\mu}{\sigma^2}}{z}{z\in [z^L,z^U]}
% \end{align*}
% Consequently, the upper bound as derived in Proposition \ref{prop:BoundCondExpect} for $z^L\geq 0$ and $z^U\rightarrow\infty$ holds. 
% \end{proof}
