# Supplementary material for: BNN-DP: Robustness Certification of Bayesian Neural Networks via Dynamic Programming
Source: arXiv:2306.10742 source file (2023-06-19)
Supplement: Supplementary file 4 [file rectified_gaussian.tex]

%% ---- RESULTS ON RECTIFIED GAUSSIAN DISTRIBUTIONS ----
\section{Rectified Gaussian Distribution}

%% ---- DEFINITION RECTIFIED GAUSSIAN DISTRIBUTION ----
% Moved to prelims

%% ---- LEMMA PROB MASS OVER RECTANGLE FOR RECTIFIED NORMAL ----
% Dropped

% \subsection*{Lemma \ref{lemma:ProbRect}}
% \begin{proof}
% \SA{All prob mass for points smaller than zero centered at zero}
% \end{proof}

%% ---- LEMMA CONVEXITY EXPECTATION RECTIFIED GAUSSIAN WRT MU & SIGMA ----
\subsection*{Lemma \ref{lemma:convexityExpectRectNormalSigmaMu}}
\begin{proof}
    Define $g:\mathbb{R}^2\rightarrow\mathbb{R}$ as
    \begin{equation}\label{eq: g}
    g(\mu,\sigma) = \frac{\mu}{2}\left[1-\erf{\frac{-\mu}{\sigma\sqrt{2}}} \right] + \frac{\sigma}{\sqrt{2\pi}}\Exp{-\frac{\mu^2}{2\sigma^2}}
    \end{equation}
    such that
    \begin{align}
    \frac{\partial g}{\partial \mu} &= \frac{1}{2}\left[1-\erf{-\frac{\mu}{\sigma\sqrt{2}}}\right] \label{eq:partial_g_partial_mu} \\
    \frac{\partial g}{\partial \sigma} &=
    \frac{1}{\sqrt{2\pi}}\Exp{-\frac{\mu^2}{2\sigma^2}} \label{eq:partial_g_partial_sigma} \\
    \frac{\partial^2g}{\partial\mu^2} &= \frac{1}{\sigma\sqrt{2\pi}}\Exp{-\frac{\mu^2}{2\sigma^2}} \nonumber\\
    \frac{\partial^2g}{\partial\sigma^2} &= \frac{\mu^2}{\sigma^3\sqrt{2\pi}}\Exp{-\frac{\mu^2}{2\sigma^2}} \nonumber\\
    \frac{\partial^2g}{\partial\sigma\partial\mu} &= -\frac{\mu}{\sigma^2\sqrt{2\pi}}\Exp{-\frac{\mu^2}{2\sigma^2}} \nonumber
    \end{align}
    Therefore, the Hessian of $g$ w.r.t. $(\mu,\sigma)$, that is, 
    \begin{align*}
    H_{(\mu,\sigma)} &= \mat{cc}{\frac{\partial^2g}{\partial\mu^2} & \frac{\partial^2g}{\partial\sigma\partial\mu} \\
    \frac{\partial^2g}{\partial\sigma\partial\mu} & \frac{\partial^2g}{\partial\sigma^2}}
    % &= \frac{1}{\sqrt{2\pi\sigma}}\Exp{-\frac{\mu^2}{2\sigma^2}}\mat{cc}{1 & \frac{1}{\sigma}\\ \frac{1}{\sigma} & \frac{1}{\sigma^2}} \\
    % &= \frac{1}{\sqrt{2\pi\sigma}}\Exp{-\frac{\mu^2}{2\sigma^2}}\mat{c}{1 & \frac{1}{\sigma}}\mat{cc}{1 & \frac{1}{\sigma}}
    % &= \frac{1}{\sqrt{2\pi\sigma}}\Exp{-\frac{\mu^2}{2\sigma^2}}cc^T
    \end{align*}
    can be written as
    $$H_{(\mu,\sigma)}= \frac{1}{\sigma\sqrt{2\pi}}\Exp{-\frac{\mu^2}{2\sigma^2}}cc^T$$
    where $c=\mat{cc}{1 & \frac{1}{\sigma}}^T\in\mathbb{R}^2$. To determine whether $H_{(\mu,\sigma)}$ is semipositive definite (spd), that is, whether $\forall z\in\mathbb{R}^2, z^TH_{(\mu,\sigma)}z$, first observe that $\forall (\mu,\sigma)\in\mathbb{R}\times\mathbb{R}_{\geq 0}$ $\frac{1}{\sqrt{2\pi\sigma}}\Exp{-\frac{\mu^2}{2\sigma^2}}\geq 0$. Second, observe that $cc^T$ is spd, because $cc^T$ is a symmetric matrix with all (leading) principal minors equal to zero. Hence, $H_{\mu,\sigma}$ is spd and, consequently, $g$ is convex w.r.t. $(\mu,\sigma)$.
\end{proof}

%% ---- LEMMA CONVEXITY EXPECTATION RECTIFIED LINEAR COMBINATION OF GAUSSIANS W.R.T. x ----
\subsection*{Lemma \ref{lemma:convexityExpectRectLinCombNormal}}
\begin{proof}
    Let $\mu(x)=\meanWeight{}{}^Tx+\meanBias{}{}$ and $\sigma^2(x)=x^T\varWeight{}{}x+\varBias{}{}^2$ with $\meanWeight{}{} \in\mathbb{R}^n$, $\meanBias{}{}\in\mathbb{R}$, $\varBias{}{}\in\mathbb{R}_{\geq0}$ and $\varWeight{}{}\in\mathbb{R}^{n\times n}$ be a semi-positive definite matrix.  
    Define $g:\mathbb{R}^n\rightarrow\mathbb{R}$ as in \eqref{eq: g}. The Hessian of $g$ w.r.t. $x$, that is,
    $H_x=\frac{\partial^2 g}{\partial x^2}$,
    % $$
    % H_x = \mat{ccc}{\frac{\partial^2 g}{\partial x^{(0)}\partial x^{(0)}} & \hdots & \frac{\partial^2 g}{\partial x^{(0)} \partial x^{(n)}} \\
    % \vdots & \ddots & \vdots \\
    % \frac{\partial^2 g}{\partial x^{(n)} \partial x^{(0)}} & \hdots & \frac{\partial^2 g}{\partial x^{(n)}\partial x^{(n)}}
    % }
    % $$
    can be written as
    $$H_x = \frac{1}{\sqrt{2\pi\sigma^2(x)}}(cc^T + \varWeight{}{} - dd^T)$$
    where, $c = \meanWeight{}{} - \frac{\mu(x)}{\sigma(x)^2}\Sigma_wx$ and $d = \frac{1}{\sigma}\Sigma_wx$. Again, to prove the convexity of $g$ w.r.t. $x$, it suffices to show that $H_x$ is spd. It can be directly concluded that $\frac{1}{\sigma(x)\sqrt{2\pi}}>0$ as $\sigma(x)>0$ and that $cc^T$ is spd since, for any $c\in \mathbb{R}^n$, $cc^T$ is a symmetric function with all (leading) principal minors equal to zero. Next, we observe that
    $$xx^T \left(\Sigma_w - \frac{\Sigma_wxx^T\Sigma_w}{x^T\Sigma_wx}\right) = O$$
    where $O\in\mathbb{R}^{n\times n}$ is the zero matrix. Here, $xx^T$ is spd by the former reasoning and by definition $O$ is spd. Then, using the result of \SA{\cite{}} that shows that the product of two symmetric psd matrices is psd, iff the product is also symmetric, we can conclude that $\Sigma_w - \frac{\Sigma_wxx^T\Sigma_w}{x^T\Sigma_wx}$ is psd. Then, because
    \begin{align*}
        \Sigma_w - dd^T &= \Sigma_w - \frac{\Sigma_wxx^T\Sigma_w}{x^T\Sigma_wx + \varBias{}{}}\\
       &\succeq \Sigma_w - \frac{\Sigma_wxx^T\Sigma_w}{x^T\Sigma_wx},
    \end{align*}
    $\Sigma_w - dd^T$ is spd. Since the sum of spd matrices is spd, $H_x$ is spd and consequently $g$ is convex w.r.t. $x$.
\end{proof}
